# Supplementary material for: Embedding Recycling for Language Models
Source: arXiv:2207.04993 source file (2023-01-30)
Supplement: Supplementary file 1 [file Early_Exiting_Results.tex]

\begin{table*}[ht]
\centering
\small
\setlength{\tabcolsep}{2.5pt}
\begin{tabular}{lcccccccccccccccc}
\toprule
                                                                          & \multicolumn{2}{c}{\textbf{Chemprot}} & \multicolumn{2}{c}{\textbf{SciCite}} & \multicolumn{2}{c}{\textbf{\begin{tabular}[c]{@{}c@{}}SciERC\\ Rel\end{tabular}}} & \multicolumn{2}{c}{\textbf{bc5cdr}} & \multicolumn{2}{c}{\textbf{JNLPBA}} & \multicolumn{2}{c}{\textbf{\begin{tabular}[c]{@{}c@{}}NCBI\\ Disease\end{tabular}}} & \multicolumn{2}{c}{\textbf{TriviaQA}} & \multicolumn{2}{c}{\textbf{SQuAD}} \\
                                                                          \cmidrule(l{7pt}r{7pt}){2-3}
                                                                         \cmidrule(l{7pt}r{7pt}){4-5}
                                                                          \cmidrule(l{7pt}r{7pt}){6-7}
                                                                          \cmidrule(l{7pt}r{7pt}){8-9}                                                  \cmidrule(l{7pt}r{7pt}){10-11}\cmidrule(l{7pt}r{7pt}){12-13}\cmidrule(l{7pt}r{7pt}){14-15}\cmidrule(l{7pt}r{7pt}){16-17}

                        & F1                & Time              & F1               & Time              & F1                                      & Time                                    & F1               & Time             & F1               & Time             & F1                                       & Time                                     & F1                & Time              & F1              & Time             \\ \midrule
\multicolumn{17}{c}{\textbf{RoBERTa-Large}}                                                                                                                                                                                                                                                                                                                                                                                                                                                 \\ \midrule
Baseline                                                                  & 84.3              & 76s               & 85.0             & 36s               & 80.2                                    & 17s                                     & 90.0             & 14min            & 79.4             & 12min            & 93                                       & 148s                                     & 78.2              & 55min             & 91.8            & 34min            \\ \cmidrule(l{7pt}r{7pt}){2-17} 
\multirow{3}{*}{\begin{tabular}[c]{@{}l@{}}Early \\ Exiting\end{tabular}} & -0.1              & -29\%             & 0.0              & -27\%             & 0.0                                     & -16\%                                   & -0.1             & -20\%            & -0.2             & -11\%            & 0.0                                      & -31\%                                    & -0.1              & -7\%              & -0.1            & -4\%             \\
                                                                          & -0.5              & -32\%             & -0.4             & -30\%             & -0.3                                    & -20\%                                   & -0.2             & -28\%            & -0.4             & -16\%            & -0.3                                     & -38\%                                    & -2.0              & -13\%             & -0.4            & -10\%            \\
                                                                          & -1.5              & 38\%              & -0.8             & -35\%             & -0.7                                    & -25\%                                   & -1.5             & -39\%            & -0.9             & -25\%            & -1.5                                     & -44\%                                    & -3.2              & -14\%             & -1.4            & -15\%            \\ \midrule
\multicolumn{17}{c}{\textbf{DeBERTa V2 XL}}                                                                                                                                                                                                                                                                                                                                                                                                                                             \\ \midrule
Baseline                                                                  & 86.8              & 131s              & 85.2             & 67s               & 79.9                                    & 30s                                     & 91.3             & 24min            & 78.5             & 22min            & 93.3                                     & 252s                                     & 80.6              & 94min             & 94.5            & 59min            \\ \cmidrule(l{7pt}r{7pt}){2-17}
\multirow{3}{*}{\begin{tabular}[c]{@{}l@{}}Early \\ Exiting\end{tabular}} & -0.4              & -10\%             & -0.3             & -15\%             & -0.6                                    & -9\%                                    & -0.1             & -4\%             & -0.1             & -2\%             & -0.2                                     & -5\%                                     & 0.0               & -5\%              & 0.0             & -4\%             \\
                                                                          & -0.8              & -14\%             & -0.6             & -18\%             & -0.8                                    & -16\%                                   & -3.2             & -12\%            & -0.3             & -3\%             & -5.4                                     & -31\%                                    & -0.8              & -7\%              & -2.0            & -9\%             \\
                                                                          & -1.5              & -18\%             & -1.4             & -22\%             & -1.0                                    & -21\%                                   & -36.1            & -47\%            & -35.0            & -45\%            & -16.3                                    & -48\%                                    & -3.4              & -11\%             & -3.3            & -12\% \\ \bottomrule           
\end{tabular}
\caption{Inference times comparison between baseline models and their reduced configurations using early exiting. For our top two performing models, RoBERTa-Large and DeBERTa V2 XL, we explored how embedding recycling could be paired with another efficiency technique, early exiting \citep{xin2020deebert}. For our early exiting testing, we used reduced models in which the earlier half of the transformer layers were removed and cached. Each column indicates varies tradeoffs between loss in F1 score and inference speedup. The percentage time improvements solely indicate inference time gains from early exiting before adding gains from embedding recycling. \jon{Review this caption}}
\label{tab:early_exiting}
\end{table*}
