# Supplementary material for: Embedding Recycling for Language Models
Source: arXiv:2207.04993 source file (2023-01-30)
Supplement: Supplementary file 2 [file HalfPrecision.tex]

\begin{table*}[ht]
\small
\centering

\setlength{\tabcolsep}{4.6pt}
\begin{tabular}{@{}lrrrrrr@{}}
\toprule
                                                                                            & \multicolumn{3}{c}{\begin{tabular}[c]{@{}c@{}}RoBERTa \\ Large\end{tabular}}                                                                                                            & \multicolumn{3}{c}{(Sci)BERT}                    
                                                                                            \\ 
                                                                                            \cmidrule(l{7pt}r{7pt}){2-4} \cmidrule(l{7pt}r{7pt}){5-7}
Task                                                                               & \multicolumn{1}{c}{\begin{tabular}[c]{@{}c@{}}Rdc\end{tabular}} & \multicolumn{1}{c}{\begin{tabular}[c]{@{}c@{}}Adpt\end{tabular}}  & \multicolumn{1}{c}{\begin{tabular}[c]{@{}c@{}}Full\end{tabular}}      & \multicolumn{1}{c}{\begin{tabular}[c]{@{}c@{}}Rdc\end{tabular}}  & \multicolumn{1}{c}{\begin{tabular}[c]{@{}c@{}}Adpt\end{tabular}} & \multicolumn{1}{c}{\begin{tabular}[c]{@{}c@{}}Full\end{tabular}}       \\ 
\midrule
 
ChemProt                                                                           & 84.3 & 84.1 & 83.9 & 84.0 & 84.2 & 84.1                         \\
SciCite                                                                            & 85.0 & 82.5 & 85.5 & 86.6 & 85.5 & 86.0                          \\
SciERC-Rel                                                                        & 80.2 & 85.7 & 80.5 & 76.7 & 86.0 & 79.8                           \\ \hdashline[1pt/1pt]
Classification Avg. & 83.2 & 84.1 & 83.3 & 82.4 & 85.2 & 83.3                        \\ \midrule
bc5cdr                                                                           & 90.0 & 90.0 & 90.4 & 90.7 & 90.0 & 91.3                 \\
JNLPBA                                                                            & 79.4 & 79.1 & 78.7  & 78.8 & 79.9 & 79.0                           \\
NCBI-disease                                                                       & 93.0 & 92.8 & 93.2 & 93.4 & 93.1  & 92.9                  \\ \hdashline[1pt/1pt]
NER Avg.                & 87.5 & 87.3 & 87.4 & 87.7 & 87.6 & 87.7      \\ \midrule
TriviaQA         & 78.2 & 78.5 & 79.8 & 67.4 & 67.4 & 69.1                 \\
SQuAD       & 91.8 & 93.5 & 93.6 & 87.5 & 87.9 & 88.4                 \\ \hdashline[1pt/1pt]
\begin{tabular}[c]{@{}l@{}}QA Avg.\end{tabular} & 85.0 & 86.0 & 86.7 & 77.5 & 77.6 & 78.8  \\ \bottomrule          
\end{tabular}
\caption{Half Precision Inference Results for Embedding Recycling. After training using full precision, we run inference for the reduced (Rdc), adapter-based (Adpt), and fully fine-tuned (Full) configurations of the RoBERTa and SciBERT models using half-precision storage. The reduced configuration corresponds to layer recycling on a reduced transformer model. The adapter-based configuration corresponds to layer recycling on a reduced frozen transformer model with added trainable Adapter modules. We find that half-precision has a negligible effect on F1-scores at inference. Error propagation rarely changes the calculated scores and when it does, it only changes rounding at the tenth decimal place. Each score represents the average score of 5 runs.
}
\label{tab:halfprecision}
\end{table*}
